# Supplementary material for: Black-Box Attacks on Sequential Recommenders via Data-Free Model Extraction
Source: arXiv:2109.01165 source file (2021-09-01)
Supplement: Supplementary file 1 [file 7_appendix.tex]

\appendix

\section{Appendix}
\subsection{Implementation Details}

\label{app:implementation}
 
\xhdr{Black-Box Model Training.} For all datasets, we treat the history of each user as a seqeuence $\bm{x} = \{x_1, x_2, \ldots, x_d\}$, where we use the first $d-2$ items $\{x_1, \ldots, x_{d-2}\}$ as training set and use the last two items for validation and testing respectively. It is worth noting that when we evaluate on the testing set, the $d-1$ previous items will be used as inputs. Optimal hyperparameters are selected using our validation set.

% \begin{table}[h]
% \begin{tabular}{@{}c|cccc@{}}
% \toprule
% \textbf{Datasets} & \textbf{Dropout} & \textbf{Hidden} & \textbf{Max. Length} & \textbf{Optimizer} \\ \midrule
% \textbf{ML-1m}    & 0.1 & 64 & 200 & AdamW \\
% \textbf{Steam}    & 0.2 & 64 & 50 & AdamW \\
% \textbf{Beauty}   & 0.5 & 64 & 50 & AdamW \\
% \bottomrule
% \end{tabular}
% \caption{Black-Box Training Details}
% \label{tab:training}
% \end{table}

We mostly follow settings of the original papers and choose the BERT4Rec setting~\cite{kang2018self} as the default in case of differences. Transformer models are initiated with $L = 2$ layers and $h = 2$ attention heads, while the NARM model has $L = 1$ layer of GRU~\cite{li2017neural}. Different sequence lengths and dropout rates of $\{0.1, 0.2, 0.5\}$ are used for the three datasets, while the hidden size is chosen to be $64$ in all cases. We train these black-box models in $128$-sized batches with an AdamW optimizer \cite{kingma2014adam, loshchilov2017decoupled}, where we take $\beta_1 = 0.9$, $\beta_2 = 0.999$ and weight decay of $0.01$. Learning rate of $0.001$ with $100$ linear warmup steps is used in black-box training, all models are trained from scratch on an NVIDIA TITAN X or RTX 2070 GPU. \textit{The relevant code and data will be released upon publication.}

\xhdr{White-Box Model Distillation.} For white-box training, most settings and hyperparameters are preserved, except that the learning rate is fixed to $0.001$.
%All sequences are split into autoregressive subsequences (i.e.,~a sequence of $\{x_1, x_2, \ldots, x_T\}$ is split into entries of $\{x_1\}, \{x_1, x_2\}, \ldots, \{x_1, x_2, \ldots, x_T\}$ \cite{li2017neural}). 
%Besides, 
To resemble real-world scenarios, only the top $100$ recommendations and their probabilities are saved while generating synthetic data using the black-box model. Therefore, it is feasible to compute the KL-Divergence loss between the recorded distribution from the black-box model and the predicted distribution of the white-box model without querying the black-box model again. Note that in order to compute the KL-Divergence loss, we only need to pick a subset of the predicted probabilities from the white-box model predictions. More precisely, only the probabilities of the same items that are recorded from the black-box model are selected to compute the KL-Divergence.

\xhdr{Adversarial Attack and Data Poisoning.} To attack the black-box model via data manipulation (Adversarial Attack) and fake profile injection (Data Poisoning), we consider 
limiting the attack with both cosine similarity and restricting the number of replaced items. In direct attack settings, less than $10\%$ of the sequence items on ML-1M could be replaced with attack items, while only $20\%$ of the elements are allowed to be attacked on Steam and Beauty, considering the shorter average sequence length. The required minimum cosine similarity between the adversarial items 
%share a minimum of $0.5$ cosine similarity
and the true item is at least $0.5$. For targeted attacks, $25$ items in total are chosen as targets according to their popularity (total appearances) in the dataset; we start from the most popular item and repeatedly pick items after a fixed distance in the popularity ranking list, so that items from the most to the least popular can be covered. We perform adversarial attacks with the mentioned targets on all test data from the ML-1M dataset, for Steam and Beauty, we randomly sample $10000$ sequences in the test set and record relevant metrics.
%with the true item. 
%While 

In the data poisoning case, other than the mentioned parameters and the autoregressive poisoning data generation in \Cref{alg:poison}, we additionally experiment on different proportions between the original data size and adversarial sample size (sequence number), in this case, we fix the adversarial sample size to be $1000$ and experiment with six different ratios of original data size: $\{0, 0.25, 0.5, 1, 2, 4\}$. Three groups of items are used as targets and we take their average metric scores to evaluate the poisoning effects. 'Top' items are defined as the first $20\%$ of items in the popularity ranking, 'mid' for items between $20\%$ and $40\%$ and 'bot' for the bottom $20\%$. We picked 10 items inside each popularity groups with fixed distance between neighbors and perform poisoning attacks on the black-box model. The retrained models are evaluated on the original test data to find out whether target items are being displayed more often.
